# Supplementary material for: Reconstructing decision trees
Source: arXiv:2012.08735 source file (2022-05-22)
Supplement: Supplementary file 1 [file appendix.tex]

\section{placeholder} 

blah blah blah
